# Supplementary material for: Temperature-dependent stability of polytypes and stacking faults in SiC: reconciling theory and experiments
Source: arXiv:1903.01936 source file (2019-03-05)
Supplement: Supplementary file 1 [file SM.pdf]

# Supplementary Material for "Temperature-dependent stability of polytypes and stacking faults in SiC: reconciling theory and experiments"

Emilio Scalise,* Anna Marzegalli, Francesco Montalenti, and Leo Miglio
*Department of Materials Science, University of Milano-Bicocca, Via Roberto Cozzi 55, 20125 Milan, IT*
(Dated: March 5, 2019)

* emilio.scalise@unimib.it

### Theoretical method

Calculations are performed using density-functional theory with PBE exchange-correlation potential [1] and including van der Waals interactions within the semiempirical method of Grimme (DFT-D2) [2], as implemented in Quantum Espresso [3]. We use a plane-wave basis set with a kinetic energy cutoff of 80 Ry, projector augmented wave (PAW) pseudopotentials [4] , and a $16 \times 16 \times 16$ Monkhorst-Pack grid for sampling the Brillouin zone of 3C-SiC, adequately reduced for larger cells. Phonon frequencies are computed through density-functional perturbation theory [5] on a $6 \times 6 \times 6$ grid (for 3C-SiC)

### Plots of the PDOS for the different SiC Polytypes

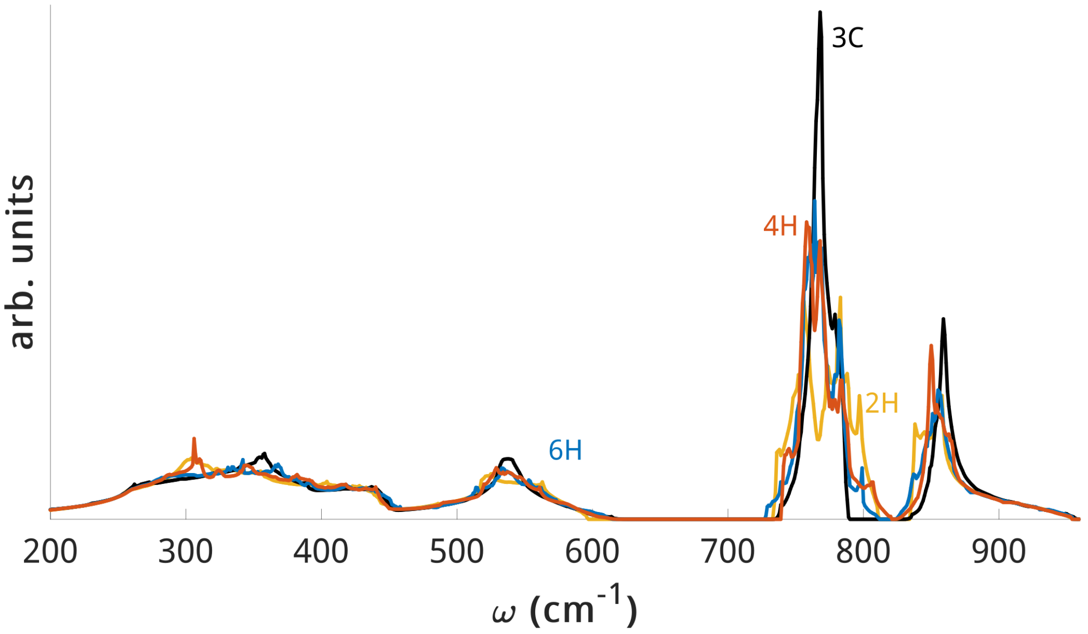


Fig. S 1. Phonon density of states (PDOS) calculated for 2H-, 4H-, 6H- and 3C-SiC.

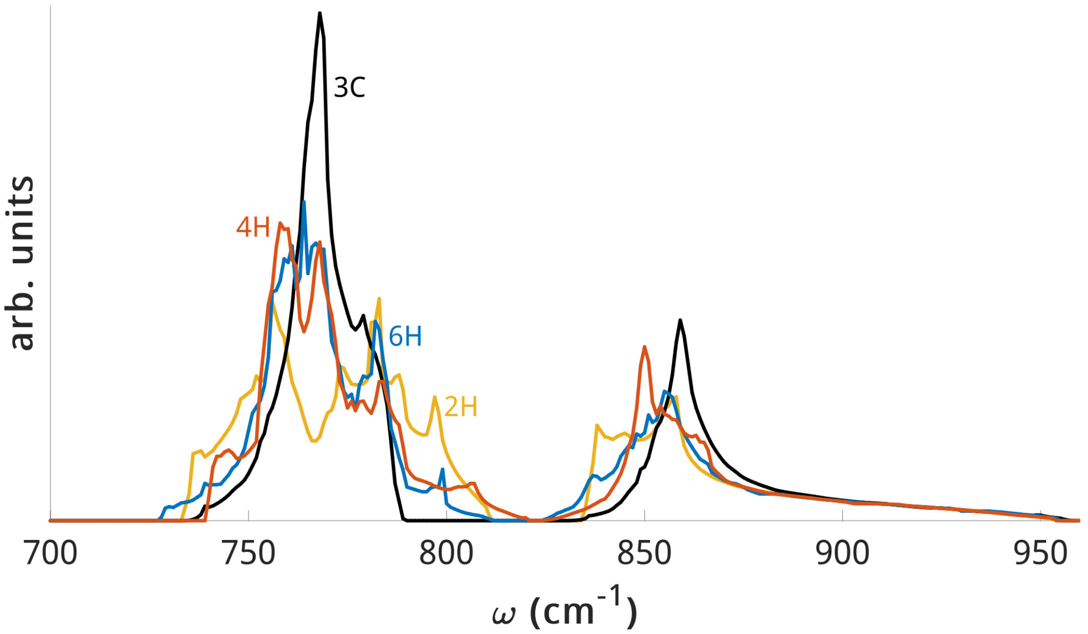


Fig. S 2. PDOS calculated for 2H-, 4H-, 6H- and 3C-SiC in the optical branches region.

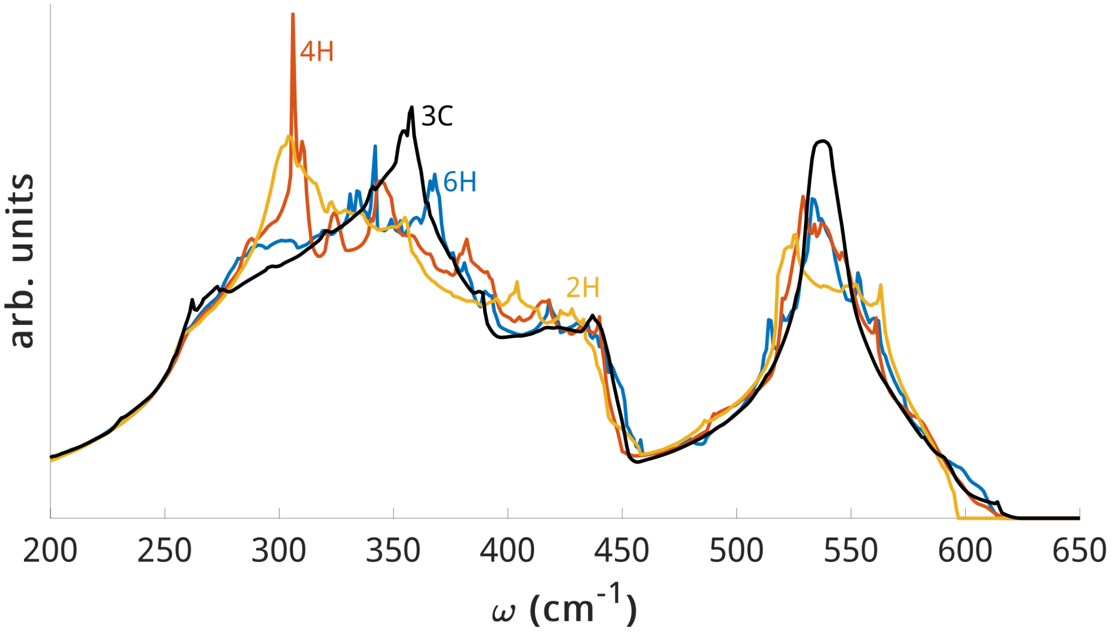


Fig. S 3. PDOS calculated for 2H-, 4H-, 6H- and 3C-SiC in the acoustic branches region

[1] J. P. Perdew, K. Burke, and M. Ernzerhof, Physical Review Letters **77**, 3865 (1996).
[2] S. Grimme, Journal of Computational Chemistry **27**, 1787 (2006).
[3] P. Giannozzi, S. Baroni, N. Bonini, M. Calandra, R. Car, C. Cavazzoni, D. Ceresoli, G. L. Chiarotti, M. Cococcioni, I. Dabo, A. Dal Corso, S. de Gironcoli, S. Fabris, G. Fratesi, R. Gebauer, U. Gerstmann, C. Gougoussis, A. Kokalj, M. Lazzeri, L. Martin-Samos, N. Marzari, F. Mauri, R. Mazzarello, S. Paolini, A. Pasquarello, L. Paulatto, C. Sbraccia, S. Scandolo, G. Sclauzero, A. P. Seitsonen, A. Smogunov, P. Umari, and R. M. Wentzcovitch, Journal of Physics: Condensed Matter **21**, 395502 (2009).
[4] P. E. Blochl, *PHYSICAL REVIEW B VOLUME*, Tech. Rep.
[5] S. Baroni, P. Giannozzi, and A. Testa, Physical Review Letters **58**, 1861 (1987).
